# Supplementary material for: Approaching optimal entangling collective measurements on quantum computing platforms
Source: arXiv:2205.15358 source file (2023-07-12)
Supplement: Supplementary file 1 [file make_fig.tex]

\documentclass[notitlepage,nofootinbib]{revtex4-1}
%\documentclass[a4]{revtex4}
%\documentclass[12pt]{iopart}
\usepackage[pdftex]{graphicx}
\usepackage{subfig}
\captionsetup{justification=RaggedRight,singlelinecheck=false,width=\linewidth,labelfont=bf,font=small}
%raggedright
%\usepackage[demo]{graphicx}
%\usepackage{caption}
%\usepackage{subcaption}
\renewcommand{\thesubfigure}{\roman{subfigure}}
\usepackage{amsmath,amsfonts,amssymb,mathtools}
%\usepackage{multicol}


\usepackage{nicematrix}
%\usepackage[margin=1in]{geometry}
\usepackage{float}
%\usepackage{mathrsfs}
\usepackage{bbm,bm}
\usepackage[normalem]{ulem}
\usepackage{color}
\usepackage{tikz}
\usetikzlibrary{shapes}
\definecolor{mycolor1}{rgb}{.9297,.5703,.6309}
\definecolor{mycolor2}{rgb}{.6212,.6114,.98575}
\definecolor{mycolor3}{rgb}{0.276,.776,.00}
\definecolor{mycolor4}{rgb}{0.98,.9203,.8809}
% \usepackage{natbib}
%\usepackage{wrapfig}
%\usepackage{natbib}
%\usepackage{apacite}
%\bibliographystyle{apacite}
%\setlength\parindent{0pt} 
%\usepackage[document]{ragged2e}

\usepackage{physics}
\usepackage{xcolor}
\newcommand{\comment}[1]{\textcolor{red}{#1}}
\newcommand{\change}[1]{\textcolor{blue}{#1}}
\pgfdeclarelayer{background}% determine background layer
\pgfsetlayers{background,main}% order of layers

 %\usepackage{biblatex}
\usepackage[utf8]{inputenc}
\usepackage{pgfplots}
\usepgfplotslibrary{groupplots}
\newcommand{\I}{\mathrm{i}}
\usepackage{lipsum}

\usepgfplotslibrary{fillbetween}

\pgfplotsset{compat=1.16}

%\input{./tikzHeaders.inc}
\def\ANU{Centre for Quantum Computation and Communication Technology, Department of Quantum Science, Australian National University, Canberra, ACT 2601, Australia.}
\def\NTU{School of Physical and Mathematical Sciences, Nanyang Technological University, Singapore 639673, Republic of Singapore}
\def\UEC{Graduate School of Informatics and Engineering, The
  University of Electro-Communications, Tokyo 182-8585, Japan}
  
\begin{document}

\title{Multiparameter estimation with two-qubit probes in noisy channels}

%\author{Lorc\'{a}n O. Conlon}
%\email{lorcan.conlon@anu.edu.au}
%\affiliation{\ANU}
%\author{Ping Koy Lam}
%\affiliation{\ANU}
%\author{Syed M Assad}
%\email{cqtsma@gmail.com}
%\affiliation{\ANU,\NTU,\UEC}


%\affiliation{Centre for Quantum Computation and Communication Technology, Department of Quantum Science,\\ Research School of Physics and Engineering, Australian National University, Canberra ACT 2601, Australia.}%
\date{\today}


\maketitle
%\tableofcontents
\section{Introduction}
%Figure: DC_dual_decoh
%\be
%Figure: AD_num_1.png
%\begin{figure}%
%\subfloat[Analytic results]{{\scalebox{.8}{\input{Amplitude_Damping_Diff_probes.tikz}}}}
%\qquad
%    \subfloat[Numerical simulations]{{\includegraphics[width=0.45\textwidth]{fig9b.png}}}%
%    \end{figure}
%    

%Fig: AD_dual_decoh
%\begin{figure}[h]
%\input{figures/AD_3par.tikz}
%\end{figure}

%Fig: AD_dual_decoh
%\begin{figure}[h]
%\input{figures/Amplitude_Damping_dual_decoh.tikz}
%\end{figure}


%Fig: AD_nag_to_hol
%\begin{figure}[h]
%  \input{figures/AD_collective_measurement.tikz}
%\end{figure}

%Fig: PD_num_1
%\begin{figure}%
%\subfloat[Analytic results]{{\scalebox{.8}{\input{PhaseDamp2q.tikz}}}}
%\qquad
%    \subfloat[Numerical simulations]{{\includegraphics[width=0.45\textwidth]{fig14b.png}}}%
%\end{figure}

%Fig: PD_dual_decoh
%\begin{figure}[h]
%\input{figures/PhaseDamp2ch.tikz}
%\end{figure}


%Fig: PD_nag_to_hol
\begin{figure}[h]
\begin{tikzpicture}
\node[right,text width=2.1cm,align=left] at (-9,5.86) {{{ (a)}}};
\node[right,text width=2.1cm,align=left] at (1.1,5.86) {{{ (b)}}};
  \begin{axis}[
    legend style={nodes={scale=1, transform shape}},
    legend cell align={left}, 
    xlabel={{Amplitude damping strength, p}}, 
    %ylabel style={align=center},ylabel= Gaussian\\non-optimality,
    ylabel style={align=left}, ylabel={{Precision}}
  %,axis lines=middle
  ,samples=100,  thick,xshift=-5cm
  ,domain=0:1
  ,ymin=0.000000,ymax=0.275,ytick={0, 0.05,0.1,0.15,0.2,0.25},yticklabels={{0},{0.05},{0.1},{0.15},{0.2},{0.25}},
xtick={0, 0.2,0.4,0.6,0.8,1},xticklabels={{0}, {0.2},{0.4},{0.6},{0.8},{1}},
,  xmin=-0.03,xmax=1.03,ylabel near ticks, xshift=-4cm,
  legend pos=north east,tick pos=left,axis line style={-},width=0.5\textwidth
  ]
\addplot[color=mycolor3,domain=0:0.5,line width=1] {0.25};
\addlegendentry{{$1/\mathcal{H}_{\text{AD}}$}}
\addplot[color=mycolor2,line width=1] {(1-x)/(4*(1-x+x^2))};
\addlegendentry{{$1/2\mathcal{N}_{2,\text{AD}} $}}
\addplot[color=mycolor1,name path=plot1q,line width=1] {(1-x)/4};
\addlegendentry{{$1/\mathcal{N}_{1,\text{AD}} $}}
\addplot[color=mycolor3,domain=0.5:1,line width=1] {(1-x)/(4*x)};
\path[name path=xaxis] (0,0) -- (1,0);
  \addplot [mycolor4] fill between [
        of=plot1q and xaxis,soft clip={domain=0:1}];
\end{axis}
\begin{axis}[width=2cm,
ylabel style={at={(-0.06,0.5)},align=center}, ylabel={{Collective--separable} \\ measurement precision gap},
xlabel={{Amplitude damping strength, p}}, width=0.5\textwidth,
legend style={at={(0.46,0.81)},anchor=south west},tick pos=left, axis line style={-},width=0.5\textwidth,
ytick={0, 0.05,0.1,0.15,0.2,0.25},yticklabels={0, 0.05,0.1,0.15,0.2,0.25}, xshift=1cm,
xmin=-0.03,xmax=1.03,ymin=0.000000,ymax=0.16,samples=100,  thick,ytick={0, 0.05,0.1,0.15,0.2,0.25},
%yticklabels={\large{0}, \large{0.05},\large{0.1},\large{0.15},\large{0.2},\large{0.25}},
yticklabels={{0},{0.05},{0.1},{0.15},{0.2},{0.25}},
xtick={0, 0.2,0.4,0.6,0.8,1},xticklabels={{0},{0.2},{0.4},{0.6},{0.8},{1}},%axis lines=left,
]
\addplot[color=mycolor2,domain=0:0.5] {0.25-(1-x)/(4*(1-x+x^2))};
\addlegendentry{{$1/\mathcal{H}_{\text{AD}}-1/2\mathcal{N}_{2,\text{AD}} $}}
\addplot[color=mycolor1,domain=0:0.5] {0.25-(1-x)/4};
\addlegendentry{{$1/\mathcal{H}_{\text{AD}}-1/\mathcal{N}_{1,\text{AD}} $}}
\addplot[color=mycolor2,domain=0.5:1] {(1-x)/(4*x)-(1-x)/(4*(1-x+x^2))};
\addplot[color=mycolor1,domain=0.5:1] {(1-x)/(4*x)-(1-x)/4};
\end{axis}
\end{tikzpicture}
\end{figure}

%Fig: Tradeoff_curve

%\begin{figure}
%\begin{tikzpicture}
%  \begin{axis}[
%    legend style={nodes={scale=1, transform shape}},
%    legend cell align={left}, 
%    xlabel=$v_x$,ylabel style={align=left}, ylabel=$v_y$
%  ,samples=100,  thick
%  ,domain=0:1
%  ,ymin=0.5,ymax=3,
%  xmin=0.5,xmax=3,ylabel near ticks,
%  legend pos=outer north east,tick pos=left, axis lines=left,axis line style={-}
%  ]
%\addplot[mark=x,black]table[x=x,y=y,col sep=comma]{data/tradeoff_dat.csv};
%\addlegendentry{$\epsilon=0.01$}
%\addplot[mark=o,red]table[x=x3,y=y3,col sep=comma]{data/tradeoff_dat.csv};
%\addlegendentry{$\epsilon=0.05$}
%\addplot[mark=*,blue]table[x=x2,y=y2,col sep=comma]{data/tradeoff_dat.csv};
%\addlegendentry{$\epsilon=0.2$}
%\end{axis}
%\end{tikzpicture}
%\end{figure}






\end{document}
